# Supplementary material for: An Actionability Assessment Tool for Explainable AI
Source: arXiv:2407.09516 source file (2024-06-19)
Supplement: Supplementary file 2 [file arc_actionabilitytool_arxiv_appendix.pdf]

# An Actionability Assessment Tool for Explainable AI

Ronal Singh, Tim Miller, Liz Sonenberg, Eduardo Velloso, Frank Vetere, Piers Howe, Paul Dourish

## APPENDIX

We follow a general MCTS algorithm [1] to generate the directives. We describe the main procedures abstractly in Alg 1, Alg 2 and Alg 2. Any off-the-shelf toolkit can be used with changes to the definitions of the nodes and reward function described in the main paper.

Before we start building the MCTS tree, we use [2] to generate one counterfactual instance,  $\vec{c}$  (line 2 of Alg 1). The counterfactual instance represents the goal state.

We then start creating the MCTS tree with a root node (ln 4 of Alg 1). This root represents the current state,  $\vec{x}$ , and does not represent any specific action,  $a$ . It also records the counterfactual state,  $\vec{c}$ , and a reference to the machine learning classifier,  $f$ . Each node in the tree has the same set of parameters. The difference between nodes is the action,  $a$ , and the resulting state,  $\vec{x}'$ . Each  $a \in A$  is a specific action taken to reach that state, and  $\vec{x}'$ , which is a set of feature values that result from taking action  $a \in A$  when in some previous state,  $\vec{x}''$ .

From the root, we carry out many episodes (ln 6 of Alg 1). The number of episodes depends on the number of actions we want to explore but could also be based on the time limitations. Each episode descends to the bottom of the tree (reaching the most promising leaf node; line 2 of Alg 2) and simulates the outcome from this leaf node by picking actions randomly (line 6 of Alg 2).

Descending the tree is done recursively. Starting from the root node *root*, the algorithm uses *Upper Confidence Bounds for Trees* (UCT) to select an action  $a \in A$ . The action,  $a$  determines the next state  $\vec{x}'$ . This process repeats until the algorithm reaches the leaf node (reaching the most promising leaf node; line 2 of Alg 2).

Once the bottom of the tree is reached, the algorithm simulates the episode (Alg 3). Actions are selected randomly (ln 22 Alg 3). This continues until a terminal state is reached (e.g. the decision has been flipped, i.e.  $f(\vec{c}) = f(\vec{x}')$ ). At this stage, the reward collected is backed up to the tree root, updating the values ( $Q$  and  $N$ ) of all relevant nodes/actions (ln 8 Alg 2).

For experiments, we set  $\alpha = 0.5$ ,  $\beta = 0.5$ , and  $\delta = [1, 10]$  (we arrived at the  $\delta$  values empirically for each scenario to get multiple trajectories for the two types of directive

explanation. From our experience,  $\delta$  is scenario- or task-dependent). The rewards were discounted by  $\gamma = 0.8$ ; this value was also arrived at empirically. Finally, we chose all categorical features and associated actions,  $A$ , to illustrate the directive explanations.

Dr Ronal Singh is with CSIRO's Data61, Melbourne, Australia  
Prof Tim Miller is with the University of Queensland, Brisbane, Australia  
Prof Liz Sonenberg, Prof Frank Vetere, and A/Prof Piers Howe are with the University of Melbourne, Melbourne, Australia  
Prof Eduardo Velloso is with the University of Sydney, Sydney, Australia  
Prof Paul Dourish is with the University of California, Irvine, US

---

**Algorithm 1:** Algorithm to generate directives

---

**Data:**  $\vec{x}, f, A$ **Result:** *directives*

```
1 /* get the counterfactual; we used
   [2] to generate 1 counterfactual
   */
2  $\vec{c} \leftarrow \text{getCounterfactual}(\vec{x})$ ;
3 /* Start building the search tree.
   The root node is always a dummy
   node without any specific action
   */
4  $\text{root} \leftarrow \text{Node}(\text{action} = \text{null}, A, \vec{x}, \vec{c})$ ;
5 /* repeat until some horizon or time
   limit. We set the horizon to the
   total number of directives */
6 for  $d$  in  $[0, \dots, \text{HORIZON}]$  do
7   /* start at the root */
8    $\text{searchNode} = \text{root}$ ;
9   /* do random rollouts */
10  for  $r$  in  $[0, \dots, \text{NUM\_ROLLOUTS}]$  do
11    /* if the current node is not a
       terminal node, i.e. decision
       has not been flipped */
12    if  $\neg \text{searchNode.isTerminal}()$  then
13      /* do rollout; this procedure
       is explained below */
14       $\text{mctsAlg.doRollout}(\text{searchNode})$ ;
15      /* choose the next best node
       to explore */
16       $\text{searchNode} \leftarrow \text{mctsAlg.choose}(\text{searchNode})$ ;
17    end
18     $r \leftarrow r + 1$ ;
19  end
20   $d \leftarrow d + 1$ ;
21 end
22 /* Get the directives. We choose the
   'cheapest' ones, that is, one with
   least cost. In case of ties, we
   pick randomly. */
23  $\text{directives} \leftarrow \text{root.getDirectives}()$ 
```

---

---

**Algorithm 2:** doRollout

---

**Data:** *searchNode***Result:** *null*

```
1 /* Use the Upper confidence bound
   (UCT) to select a child node to
   explore */
2  $\text{leafNode} \leftarrow \text{uctSelect}(\text{searchNode})$ ;
3 /* expand the leaf node; add the
   children of the leaf node to the
   tree and for each child node, add
   the action represented by the node
   and the new state,  $\mathbf{x}'$  that results
   after applying the node's action,
    $a$ . */
4  $\text{leafNode.expand}()$ ;
5 /* simulate and get the reward for
   the leaf node; algorithm provided
   later. */
6  $\text{reward} = \text{self.simulate}(\text{leaf})$ ;
7 /* backpropagate the reward; update
   the  $Q$  and  $\mathcal{N}$  */
8  $\text{leaf.backpropagate}(\text{reward})$ 
```

---

---

**Algorithm 3:** simulate

---

**Data:**  $leaf, \vec{x}, f$ **Result:**  $reward$ 

```
1  $node \leftarrow leaf$ ;
2 while  $true$  do
3   /*  $isTerminal()$  returns True if the
   decision has been flipped. */
4   if  $node.isTerminal()$  then
5     /* get the vector of feature
       values representing the
       current state */
6      $\vec{x}' \leftarrow getState(node)$ ;
7     /* get counterfactual state */
8      $\vec{c} \leftarrow getCounterfactualState(node)$ ;
9     /* compute the Euclidean
       distance between  $\vec{c}$  and  $\vec{x}'$  */
10     $distance = euclideanDistance(\vec{c}, \vec{x}')$ ;
11    /* get the desired
       outcome/decision */
12     $y' \leftarrow f(\vec{c})$ ;
13    /* initialise the reward to zero
       */
14     $reward \leftarrow 0$ ;
15    /* If the distance between  $\vec{x}$  and
        $\vec{x}'$  is within user specified
       range,  $\delta$ , and the decision is
       flipped,  $y' = f(\vec{x}')$ , then
       compute and return the
       reward. Otherwise, reward is
       ZERO. While we return the
       reward for the node that
       meets the following criteria,
       note that actions before this
       node would have changed the
       state  $\vec{x}'$ , and this node
       represents the state that we
       reached as a result of
       applying all actions leading
       up to and including this
       node. */
16    if  $distance \leq \delta$  &  $y' = f(\vec{x}')$  then
17      |  $reward \leftarrow (\alpha + \beta) * \gamma$ ;
18    end
19     $return\ reward$ ;
20  end
21  /* keep traversing/expanding the
     tree, each time choosing a
     random child/action. */
22   $node \leftarrow node.findRandomChild()$ ;
23  /* no more nodes to explore */
24  if  $node = null$  then
25    |  $return\ 0.0$ ;
26  end
27 end
```

---

### Loan Applicant Profile

| Feature                      | Value          |
|------------------------------|----------------|
| Loan Amount (\$)             | 3000           |
| Loan Term (months)           | 36             |
| Interest Rate (%)            | 15.6           |
| Credit Rating                | C              |
| Salary                       | 30000          |
| Work Experience (years)      | 8              |
| Credit Utilisation Rate (%)  | 29             |
| Debt to Income Ratio (%)     | 16.44          |
| Delinquencies (last 2 years) | 0              |
| <b>DECISION:</b>             | <b>APPROVE</b> |

Your details were supplied to a credit-scoring algorithm that approved your loan application based on your credit utilisation rate of 29%.

We assess:

- Credit Rating on a scale of A to F where A is an excellent rating, and F is for a poor rating.
- Credit Utilisation Rate: measures how much credit a customer is using compared with how much the customer has available, expressed as a percentage
- Debt to Income Ratio is calculated by dividing total recurring monthly debt by monthly gross income.

Fig. 1. Study 1: Sample scenario.

### Question:

The system has generated the following two explanations for you. Which of the two explanations do you think is more actionable?

We would have DENIED you the loan if your credit utilisation rate was worse than your current utilisation rate. If your credit utilisation rate had been higher than 30%, we would have denied you the loan.

We would have DENIED you the loan if your credit utilisation rate was higher than 30%. If you kept on using your credit card without paying them off, you could increase your credit utilisation rate to 30%

Fig. 2. Study 1: Sample question for scenario shown in Fig 1.

### Loan Applicant Profile

| Feature                      | Value       |
|------------------------------|-------------|
| Loan Amount (\$)             | 5600        |
| Loan Term (months)           | 60          |
| Interest Rate (%)            | 21.5        |
| Credit Rating                | F           |
| Salary                       | 40000       |
| Work Experience (years)      | 4           |
| Credit Utilisation Rate (%)  | 32.6        |
| Debt to Income Ratio (%)     | 27          |
| Delinquencies (last 2 years) | 0           |
| <b>DECISION:</b>             | <b>DENY</b> |

Your details were supplied to a credit-scoring algorithm that decided to deny your loan application based on your credit rating. You have a credit rating of F on a scale of A to F, where A is an excellent rating and F is a poor rating.

We assess:

- Credit Rating on a scale of A to F where A is an excellent rating, and F is for a poor rating.
- Credit Utilisation Rate: measures how much credit a customer is using compared with how much the customer has available, expressed as a percentage
- Debt to Income Ratio is calculated by dividing total recurring monthly debt by monthly gross income.

### Explanation:

The system has generated the following explanation for you (as the loan applicant):

*To change the decision to APPROVE, your credit rating needs to be at least C.*

Fig. 3. Study 2: Sample scenario.

Please answer the following questions for the **explanation** generated by the AI for you (as the loan applicant).

not at all      always  
0      1      2      3      4      5      6      7      8      9      10

The information is clear and easy to understand.

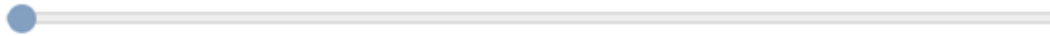

The information helps me understand the reason(s) for the decision/prediction.

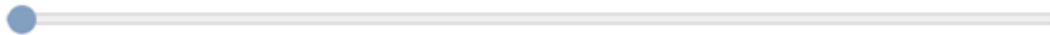

The information is relevant to my personal circumstances.

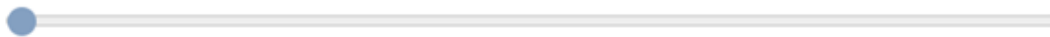

The information is socially appropriate.

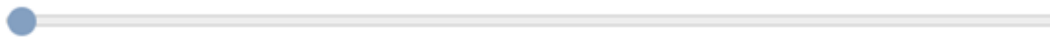

The information allows me to identify and correct any misunderstandings of my personal situation.

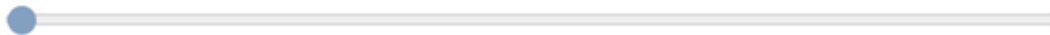

The information allows me to identify at least one feasible action to achieve my desired outcome.

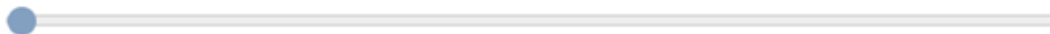

The information allows me to break down any action into explicit steps.

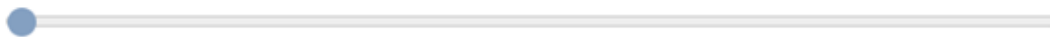

Fig. 4. Study 2: Sample questions for scenario shown in Fig 3.

| Employee: Tanya                                                                                                                                                                                                                                                                                                                                                                                                                                                                                                                                                                                                                                                                                                                                                                                                                                                                                                                                                                                                                                                                                                                                                                                                                                                                  |                   |
|----------------------------------------------------------------------------------------------------------------------------------------------------------------------------------------------------------------------------------------------------------------------------------------------------------------------------------------------------------------------------------------------------------------------------------------------------------------------------------------------------------------------------------------------------------------------------------------------------------------------------------------------------------------------------------------------------------------------------------------------------------------------------------------------------------------------------------------------------------------------------------------------------------------------------------------------------------------------------------------------------------------------------------------------------------------------------------------------------------------------------------------------------------------------------------------------------------------------------------------------------------------------------------|-------------------|
| Feature                                                                                                                                                                                                                                                                                                                                                                                                                                                                                                                                                                                                                                                                                                                                                                                                                                                                                                                                                                                                                                                                                                                                                                                                                                                                          | Value             |
| Age                                                                                                                                                                                                                                                                                                                                                                                                                                                                                                                                                                                                                                                                                                                                                                                                                                                                                                                                                                                                                                                                                                                                                                                                                                                                              | 43                |
| Business Travel                                                                                                                                                                                                                                                                                                                                                                                                                                                                                                                                                                                                                                                                                                                                                                                                                                                                                                                                                                                                                                                                                                                                                                                                                                                                  | Medium            |
| Employment length (in the company)                                                                                                                                                                                                                                                                                                                                                                                                                                                                                                                                                                                                                                                                                                                                                                                                                                                                                                                                                                                                                                                                                                                                                                                                                                               | 4 years           |
| Employment length (lifetime)                                                                                                                                                                                                                                                                                                                                                                                                                                                                                                                                                                                                                                                                                                                                                                                                                                                                                                                                                                                                                                                                                                                                                                                                                                                     | 7 years           |
| Months since last promotion                                                                                                                                                                                                                                                                                                                                                                                                                                                                                                                                                                                                                                                                                                                                                                                                                                                                                                                                                                                                                                                                                                                                                                                                                                                      | 12                |
| Monthly income (\$)                                                                                                                                                                                                                                                                                                                                                                                                                                                                                                                                                                                                                                                                                                                                                                                                                                                                                                                                                                                                                                                                                                                                                                                                                                                              | 5300              |
| Overtime status                                                                                                                                                                                                                                                                                                                                                                                                                                                                                                                                                                                                                                                                                                                                                                                                                                                                                                                                                                                                                                                                                                                                                                                                                                                                  | Yes               |
| Coworker relationship satisfaction                                                                                                                                                                                                                                                                                                                                                                                                                                                                                                                                                                                                                                                                                                                                                                                                                                                                                                                                                                                                                                                                                                                                                                                                                                               | Very dissatisfied |
| Job involvement                                                                                                                                                                                                                                                                                                                                                                                                                                                                                                                                                                                                                                                                                                                                                                                                                                                                                                                                                                                                                                                                                                                                                                                                                                                                  | Disengaged        |
| Work environment satisfaction                                                                                                                                                                                                                                                                                                                                                                                                                                                                                                                                                                                                                                                                                                                                                                                                                                                                                                                                                                                                                                                                                                                                                                                                                                                    | Very dissatisfied |
| <b>PREDICTION:</b>                                                                                                                                                                                                                                                                                                                                                                                                                                                                                                                                                                                                                                                                                                                                                                                                                                                                                                                                                                                                                                                                                                                                                                                                                                                               | <b>RESIGN</b>     |
| <p>Tanya's details were supplied to an automated system used by the Human Resources Department that predicted that Tanya would likely <b>resign</b> due to multiple factors, which includes dissatisfaction with her relationship with her co-workers, her low job involvement levels, and increased overtime. At present, Tanya does overtime, her co-worker relationship satisfaction is 'very dissatisfied' and her job involvement level is 'disengaged'. These ratings are due to an increase in business-related travel, which added overtime and took time away that Tanya usually spends with her colleagues.</p> <p>We assess:</p> <ul style="list-style-type: none"> <li>• overtime on a 2-point scale: Yes (does overtime), and No (does not do overtime)</li> <li>• co-worker relationship satisfaction on a 4-point scale: from very dissatisfied, dissatisfied, satisfied, and very satisfied.</li> <li>• job involvement levels on a 4-point scale: highly disengaged, disengaged, engaged, and very engaged.</li> <li>• business travel on a 3-point scale: Low (0 – 1 per month), Medium (2 – 3), and High (4 or more).</li> <li>• work environment satisfaction on a 4-point scale: very dissatisfied, dissatisfied, satisfied, and very satisfied.</li> </ul> |                   |
| <p><b>Counterfactual explanation:</b> To change the prediction to STAY, you need to change Tanya's overtime status to 'No', her co-worker relationship satisfaction to 'satisfied' and her job involvement level to 'engaged'.</p>                                                                                                                                                                                                                                                                                                                                                                                                                                                                                                                                                                                                                                                                                                                                                                                                                                                                                                                                                                                                                                               |                   |
| <p><b>Directive explanation:</b> To change the prediction to STAY, change Tanya's overtime status to 'No', her co-worker relationship satisfaction to 'satisfied', and her job involvement level to 'engaged'. To do these, you could hire one casual staff to support Tanya and organise a workers' retreat for Tanya and her colleagues.</p>                                                                                                                                                                                                                                                                                                                                                                                                                                                                                                                                                                                                                                                                                                                                                                                                                                                                                                                                   |                   |
| <p><b>Prototypical explanation:</b> The following is an example of an employee who is likely to STAY (not resign):</p>                                                                                                                                                                                                                                                                                                                                                                                                                                                                                                                                                                                                                                                                                                                                                                                                                                                                                                                                                                                                                                                                                                                                                           |                   |
| Employee: Prototype                                                                                                                                                                                                                                                                                                                                                                                                                                                                                                                                                                                                                                                                                                                                                                                                                                                                                                                                                                                                                                                                                                                                                                                                                                                              |                   |
| Feature                                                                                                                                                                                                                                                                                                                                                                                                                                                                                                                                                                                                                                                                                                                                                                                                                                                                                                                                                                                                                                                                                                                                                                                                                                                                          | Value             |
| Age                                                                                                                                                                                                                                                                                                                                                                                                                                                                                                                                                                                                                                                                                                                                                                                                                                                                                                                                                                                                                                                                                                                                                                                                                                                                              | 29                |
| Business Travel                                                                                                                                                                                                                                                                                                                                                                                                                                                                                                                                                                                                                                                                                                                                                                                                                                                                                                                                                                                                                                                                                                                                                                                                                                                                  | Medium            |
| Employment length (in the company)                                                                                                                                                                                                                                                                                                                                                                                                                                                                                                                                                                                                                                                                                                                                                                                                                                                                                                                                                                                                                                                                                                                                                                                                                                               | 5 years           |
| Employment length (lifetime)                                                                                                                                                                                                                                                                                                                                                                                                                                                                                                                                                                                                                                                                                                                                                                                                                                                                                                                                                                                                                                                                                                                                                                                                                                                     | 6 years           |
| Months since last promotion                                                                                                                                                                                                                                                                                                                                                                                                                                                                                                                                                                                                                                                                                                                                                                                                                                                                                                                                                                                                                                                                                                                                                                                                                                                      | 0                 |
| Monthly income (\$)                                                                                                                                                                                                                                                                                                                                                                                                                                                                                                                                                                                                                                                                                                                                                                                                                                                                                                                                                                                                                                                                                                                                                                                                                                                              | 2700              |
| Overtime status                                                                                                                                                                                                                                                                                                                                                                                                                                                                                                                                                                                                                                                                                                                                                                                                                                                                                                                                                                                                                                                                                                                                                                                                                                                                  | No                |
| Coworker relationship satisfaction                                                                                                                                                                                                                                                                                                                                                                                                                                                                                                                                                                                                                                                                                                                                                                                                                                                                                                                                                                                                                                                                                                                                                                                                                                               | Very satisfied    |
| Job involvement                                                                                                                                                                                                                                                                                                                                                                                                                                                                                                                                                                                                                                                                                                                                                                                                                                                                                                                                                                                                                                                                                                                                                                                                                                                                  | Engaged           |
| Work environment satisfaction                                                                                                                                                                                                                                                                                                                                                                                                                                                                                                                                                                                                                                                                                                                                                                                                                                                                                                                                                                                                                                                                                                                                                                                                                                                    | Satisfied         |
| <b>PREDICTION:</b>                                                                                                                                                                                                                                                                                                                                                                                                                                                                                                                                                                                                                                                                                                                                                                                                                                                                                                                                                                                                                                                                                                                                                                                                                                                               | <b>STAY</b>       |

TABLE I  
EMPLOYEE TURNOVER SCENARIO 1

| Employee: Mel                                                                                                                                                                                                                                                                                            |                 |
|----------------------------------------------------------------------------------------------------------------------------------------------------------------------------------------------------------------------------------------------------------------------------------------------------------|-----------------|
| Feature                                                                                                                                                                                                                                                                                                  | Value           |
| Age                                                                                                                                                                                                                                                                                                      | 26              |
| Business Travel                                                                                                                                                                                                                                                                                          | Low             |
| Employment length (in the company)                                                                                                                                                                                                                                                                       | 2 years         |
| Employment length (lifetime)                                                                                                                                                                                                                                                                             | 7 years         |
| Months since last promotion                                                                                                                                                                                                                                                                              | 24              |
| Monthly income (\$)                                                                                                                                                                                                                                                                                      | 4900            |
| Overtime status                                                                                                                                                                                                                                                                                          | No              |
| Coworker relationship satisfaction                                                                                                                                                                                                                                                                       | Very satisfied  |
| Job involvement                                                                                                                                                                                                                                                                                          | Very disengaged |
| Work environment satisfaction                                                                                                                                                                                                                                                                            | Dissatisfied    |
| <b>PREDICTION:</b>                                                                                                                                                                                                                                                                                       | <b>RESIGN</b>   |
| <p>Mel's details were supplied to an automated system used by the Human Resources Department that predicted that Mel would likely resign because she is 'very dissatisfied' with her work environment. This dissatisfaction may have been due to the recent increase in her business-related travel.</p> |                 |
| <p><b>Counterfactual explanation:</b> To change the prediction to STAY, you need to change Mel's work environment satisfaction to at least 'satisfied'.</p>                                                                                                                                              |                 |
| <p><b>Directive explanation:</b> To change the prediction to STAY, change Mel's work environment satisfaction to 'satisfied'. To do this, you could provide her with one business class travel per month.</p>                                                                                            |                 |
| <p><b>Prototypical explanation:</b> The following is an example of an employee who is likely to STAY (not resign):</p>                                                                                                                                                                                   |                 |
| Employee: Prototype                                                                                                                                                                                                                                                                                      |                 |
| Feature                                                                                                                                                                                                                                                                                                  | Value           |
| Age                                                                                                                                                                                                                                                                                                      | 29              |
| Business Travel                                                                                                                                                                                                                                                                                          | Medium          |
| Employment length (in the company)                                                                                                                                                                                                                                                                       | 5 years         |
| Employment length (lifetime)                                                                                                                                                                                                                                                                             | 6 years         |
| Months since last promotion                                                                                                                                                                                                                                                                              | 0               |
| Monthly income (\$)                                                                                                                                                                                                                                                                                      | 2700            |
| Overtime status                                                                                                                                                                                                                                                                                          | No              |
| Coworker relationship satisfaction                                                                                                                                                                                                                                                                       | Very satisfied  |
| Job involvement                                                                                                                                                                                                                                                                                          | Engaged         |
| Work environment satisfaction                                                                                                                                                                                                                                                                            | Satisfied       |
| <b>PREDICTION:</b>                                                                                                                                                                                                                                                                                       | <b>STAY</b>     |

TABLE II  
EMPLOYEE TURNOVER SCENARIO 2



| Employee: Scott                                                                                                                                                                                                                                                                                                                         |                |
|-----------------------------------------------------------------------------------------------------------------------------------------------------------------------------------------------------------------------------------------------------------------------------------------------------------------------------------------|----------------|
| Feature                                                                                                                                                                                                                                                                                                                                 | Value          |
| Age                                                                                                                                                                                                                                                                                                                                     | 43             |
| Business Travel                                                                                                                                                                                                                                                                                                                         | Low            |
| Employment length (in the company)                                                                                                                                                                                                                                                                                                      | 4 years        |
| Employment length (lifetime)                                                                                                                                                                                                                                                                                                            | 7 years        |
| Months since last promotion                                                                                                                                                                                                                                                                                                             | 24             |
| Monthly income (\$)                                                                                                                                                                                                                                                                                                                     | 2100           |
| Overtime status                                                                                                                                                                                                                                                                                                                         | No             |
| Coworker relationship satisfaction                                                                                                                                                                                                                                                                                                      | Very satisfied |
| Job involvement                                                                                                                                                                                                                                                                                                                         | Very engaged   |
| Work environment satisfaction                                                                                                                                                                                                                                                                                                           | Very satisfied |
| <b>PREDICTION:</b>                                                                                                                                                                                                                                                                                                                      | <b>STAY</b>    |
| Scott's details were supplied to an automated system used by the Human Resources Department that predicted that Scott is NOT likely to resign in the near future because his business travel is 'low', job involvement is 'very engaged', and environment satisfaction is 'very satisfied' (see scales below).                          |                |
| <b>Counterfactual explanation:</b> Scott may resign if his travel were to change to 'high', environment satisfaction was to change to 'dissatisfied', and his job involvement was to change to 'disengaged'.                                                                                                                            |                |
| <b>Directive explanation:</b> Scott may resign if his travel changed to 'high', environment satisfaction to 'dissatisfied' and job involvement to 'disengaged'. This could happen if he stopped doing online client meetings (and doing more in-person meetings) and if you stopped the quarterly meetings to discuss his career plans. |                |
| <b>Prototypical explanation:</b> The following employee is likely to RESIGN:                                                                                                                                                                                                                                                            |                |
| Employee: Prototype                                                                                                                                                                                                                                                                                                                     |                |
| Feature                                                                                                                                                                                                                                                                                                                                 | Value          |
| Age                                                                                                                                                                                                                                                                                                                                     | 36             |
| Business Travel                                                                                                                                                                                                                                                                                                                         | High           |
| Employment length (in the company)                                                                                                                                                                                                                                                                                                      | 8 years        |
| Employment length (lifetime)                                                                                                                                                                                                                                                                                                            | 13 years       |
| Months since last promotion                                                                                                                                                                                                                                                                                                             | 96             |
| Monthly income (\$)                                                                                                                                                                                                                                                                                                                     | 2000           |
| Overtime status                                                                                                                                                                                                                                                                                                                         | No             |
| Coworker relationship satisfaction                                                                                                                                                                                                                                                                                                      | Satisfied      |
| Job involvement                                                                                                                                                                                                                                                                                                                         | Engaged        |
| Work environment satisfaction                                                                                                                                                                                                                                                                                                           | Satisfied      |
| <b>PREDICTION:</b>                                                                                                                                                                                                                                                                                                                      | <b>RESIGN</b>  |

TABLE III  
EMPLOYEE TURNOVER SCENARIO 3

| Employee: Belinda                                                                                                                                                                                                                                                                                                                                                                                       |                |
|---------------------------------------------------------------------------------------------------------------------------------------------------------------------------------------------------------------------------------------------------------------------------------------------------------------------------------------------------------------------------------------------------------|----------------|
| Feature                                                                                                                                                                                                                                                                                                                                                                                                 | Value          |
| Age                                                                                                                                                                                                                                                                                                                                                                                                     | 40             |
| Business Travel                                                                                                                                                                                                                                                                                                                                                                                         | Medium         |
| Employment length (in the company)                                                                                                                                                                                                                                                                                                                                                                      | 9 years        |
| Employment length (lifetime)                                                                                                                                                                                                                                                                                                                                                                            | 9 years        |
| Months since last promotion                                                                                                                                                                                                                                                                                                                                                                             | 48             |
| Monthly income (\$)                                                                                                                                                                                                                                                                                                                                                                                     | 3300           |
| Overtime status                                                                                                                                                                                                                                                                                                                                                                                         | No             |
| Coworker relationship satisfaction                                                                                                                                                                                                                                                                                                                                                                      | Very satisfied |
| Job involvement                                                                                                                                                                                                                                                                                                                                                                                         | Engaged        |
| Work environment satisfaction                                                                                                                                                                                                                                                                                                                                                                           | Very satisfied |
| <b>PREDICTION:</b>                                                                                                                                                                                                                                                                                                                                                                                      | <b>STAY</b>    |
| <p>Belinda's details were supplied to an automated system used by the Human Resources Department that predicted that Belinda is NOT likely to resign in the near future because she has not done overtime. Also because she attends all of the departments social activities, her co-worker relationship satisfaction is 'very satisfied', and her job involvement is 'engaged' (see scales below).</p> |                |
| <p><b>Counterfactual explanation:</b> Belinda may resign if her overtime status and job involvement levels changed, that is, if she were to do overtime, her co-worker relationship satisfaction changed to 'dissatisfied', and her job involvement level changed to 'disengaged'.</p>                                                                                                                  |                |
| <p><b>Directive explanation:</b> Belinda may resign if she were to do overtime, her co-worker relationship satisfaction became 'dissatisfied', and her job involvement level became 'disengaged'. This could happen if Belinda stopped attending the weekly departmental meetings and coffees.</p>                                                                                                      |                |
| <b>Prototypical explanation:</b> The following employee is likely to RESIGN:                                                                                                                                                                                                                                                                                                                            |                |
| Employee: Prototype                                                                                                                                                                                                                                                                                                                                                                                     |                |
| Feature                                                                                                                                                                                                                                                                                                                                                                                                 | Value          |
| Age                                                                                                                                                                                                                                                                                                                                                                                                     | 36             |
| Business Travel                                                                                                                                                                                                                                                                                                                                                                                         | High           |
| Employment length (in the company)                                                                                                                                                                                                                                                                                                                                                                      | 8 years        |
| Employment length (lifetime)                                                                                                                                                                                                                                                                                                                                                                            | 13 years       |
| Months since last promotion                                                                                                                                                                                                                                                                                                                                                                             | 96             |
| Monthly income (\$)                                                                                                                                                                                                                                                                                                                                                                                     | 2000           |
| Overtime status                                                                                                                                                                                                                                                                                                                                                                                         | No             |
| Coworker relationship satisfaction                                                                                                                                                                                                                                                                                                                                                                      | Satisfied      |
| Job involvement                                                                                                                                                                                                                                                                                                                                                                                         | Engaged        |
| Work environment satisfaction                                                                                                                                                                                                                                                                                                                                                                           | Satisfied      |
| <b>PREDICTION:</b>                                                                                                                                                                                                                                                                                                                                                                                      | <b>RESIGN</b>  |

TABLE IV  
EMPLOYEE TURNOVER SCENARIO 4

| Applicant Profile                                                                                                                                                                                                                                                                                                                                                                                                                                                                                                                                                                                                                                                                                     |                |
|-------------------------------------------------------------------------------------------------------------------------------------------------------------------------------------------------------------------------------------------------------------------------------------------------------------------------------------------------------------------------------------------------------------------------------------------------------------------------------------------------------------------------------------------------------------------------------------------------------------------------------------------------------------------------------------------------------|----------------|
| Feature                                                                                                                                                                                                                                                                                                                                                                                                                                                                                                                                                                                                                                                                                               | Value          |
| Loan Amount (\$)                                                                                                                                                                                                                                                                                                                                                                                                                                                                                                                                                                                                                                                                                      | 5600           |
| Loan Term (months)                                                                                                                                                                                                                                                                                                                                                                                                                                                                                                                                                                                                                                                                                    | 60             |
| Interest Rate (%)                                                                                                                                                                                                                                                                                                                                                                                                                                                                                                                                                                                                                                                                                     | 21.5           |
| Credit Rating                                                                                                                                                                                                                                                                                                                                                                                                                                                                                                                                                                                                                                                                                         | F              |
| Salary                                                                                                                                                                                                                                                                                                                                                                                                                                                                                                                                                                                                                                                                                                | 40000          |
| Work Experience (years)                                                                                                                                                                                                                                                                                                                                                                                                                                                                                                                                                                                                                                                                               | 4              |
| Credit Utilisation Rate (%)                                                                                                                                                                                                                                                                                                                                                                                                                                                                                                                                                                                                                                                                           | 32.6           |
| Debt to Income Ratio (%)                                                                                                                                                                                                                                                                                                                                                                                                                                                                                                                                                                                                                                                                              | 27             |
| Delinquencies (last 2 years)                                                                                                                                                                                                                                                                                                                                                                                                                                                                                                                                                                                                                                                                          | 0              |
| <b>DECISION:</b>                                                                                                                                                                                                                                                                                                                                                                                                                                                                                                                                                                                                                                                                                      | <b>DENY</b>    |
| <p>Your details were supplied to a credit-scoring algorithm that decided to deny your loan application based on your credit rating. You have a credit rating of F on a scale of A to F, where A is an excellent rating and F is a poor rating.</p> <p>We assess:</p> <ul style="list-style-type: none"> <li>• Credit Rating on a scale of A to F where A is an excellent rating, and F is for a poor rating.</li> <li>• Credit Utilisation Rate: measures how much credit a customer is using compared with how much the customer has available, expressed as a percentage</li> <li>• Debt to Income Ratio is calculated by dividing total recurring monthly debt by monthly gross income.</li> </ul> |                |
| <p><b>Counterfactual explanation:</b> To change the decision to APPROVE, your credit rating needs to be at least C.</p>                                                                                                                                                                                                                                                                                                                                                                                                                                                                                                                                                                               |                |
| <p><b>Directive explanation:</b> To change the decision to APPROVE, your credit rating needs to be C. You could get a credit rating of C in six months if you were to enable automatic deductions from your savings account to make the monthly credit card payments on time.</p>                                                                                                                                                                                                                                                                                                                                                                                                                     |                |
| <p><b>Prototypical explanation:</b> The following is an example of an APPROVED applicant:</p>                                                                                                                                                                                                                                                                                                                                                                                                                                                                                                                                                                                                         |                |
| Applicant Profile                                                                                                                                                                                                                                                                                                                                                                                                                                                                                                                                                                                                                                                                                     |                |
| Feature                                                                                                                                                                                                                                                                                                                                                                                                                                                                                                                                                                                                                                                                                               | Value          |
| Loan Amount (\$)                                                                                                                                                                                                                                                                                                                                                                                                                                                                                                                                                                                                                                                                                      | 16000          |
| Loan Term (months)                                                                                                                                                                                                                                                                                                                                                                                                                                                                                                                                                                                                                                                                                    | 36             |
| Interest Rate (%)                                                                                                                                                                                                                                                                                                                                                                                                                                                                                                                                                                                                                                                                                     | 12.18          |
| Credit Rating                                                                                                                                                                                                                                                                                                                                                                                                                                                                                                                                                                                                                                                                                         | B              |
| Salary                                                                                                                                                                                                                                                                                                                                                                                                                                                                                                                                                                                                                                                                                                | 120000         |
| Work Experience (years)                                                                                                                                                                                                                                                                                                                                                                                                                                                                                                                                                                                                                                                                               | 8              |
| Credit Utilisation Rate (%)                                                                                                                                                                                                                                                                                                                                                                                                                                                                                                                                                                                                                                                                           | 70             |
| Debt to Income Ratio (%)                                                                                                                                                                                                                                                                                                                                                                                                                                                                                                                                                                                                                                                                              | 21             |
| Delinquencies (last 2 years)                                                                                                                                                                                                                                                                                                                                                                                                                                                                                                                                                                                                                                                                          | 0              |
| <b>DECISION:</b>                                                                                                                                                                                                                                                                                                                                                                                                                                                                                                                                                                                                                                                                                      | <b>APPROVE</b> |

TABLE V  
CREDIT SCENARIO 1

## REFERENCES

- [1] C. B. Browne, E. Powley, D. Whitehouse, S. M. Lucas, P. I. Cowling, P. Rohlfshagen, S. Tavener, D. Perez, S. Samothrakis, and S. Colton, "A survey of monte carlo tree search methods," *IEEE Trans. Comput. Intell. AI Games*, vol. 4, no. 1, pp. 1–43, Mar. 2012.
- [2] C. Russell, "Efficient search for diverse coherent explanations," in *Proceedings of the Conference on Fairness, Accountability, and Transparency*, ser. FAT\* '19. New York, NY, USA: Association for Computing Machinery, Jan. 2019, pp. 20–28.

| Applicant Profile                                                                                                                                                                                           |                |
|-------------------------------------------------------------------------------------------------------------------------------------------------------------------------------------------------------------|----------------|
| Feature                                                                                                                                                                                                     | Value          |
| Loan Amount (\$)                                                                                                                                                                                            | 11000          |
| Loan Term (months)                                                                                                                                                                                          | 36             |
| Interest Rate (%)                                                                                                                                                                                           | 16.5           |
| Credit Rating                                                                                                                                                                                               | D              |
| Salary                                                                                                                                                                                                      | 38000          |
| Work Experience (years)                                                                                                                                                                                     | 4              |
| Credit Utilisation Rate (%)                                                                                                                                                                                 | 43.4           |
| Debt to Income Ratio (%)                                                                                                                                                                                    | 7.35           |
| Delinquencies (last 2 years)                                                                                                                                                                                | 0              |
| <b>DECISION:</b>                                                                                                                                                                                            | <b>DENY</b>    |
| Your details were supplied to a credit-scoring algorithm that decided to deny your loan application based on your income.                                                                                   |                |
| <b>Counterfactual explanation:</b> To change the decision to APPROVE, your income needs to be higher than \$42000. If your income had been above \$42000, we could have given you a loan.                   |                |
| <b>Directive explanation:</b> To change the decision to APPROVE, your income needs to be higher than \$42000. You could increase your income by getting a promotion, a secondary job, or finding a new job. |                |
| <b>Prototypical explanation:</b> The following is an example of an APPROVED applicant:                                                                                                                      |                |
| Applicant Profile                                                                                                                                                                                           |                |
| Feature                                                                                                                                                                                                     | Value          |
| Loan Amount (\$)                                                                                                                                                                                            | 16000          |
| Loan Term (months)                                                                                                                                                                                          | 36             |
| Interest Rate (%)                                                                                                                                                                                           | 12.18          |
| Credit Rating                                                                                                                                                                                               | B              |
| Salary                                                                                                                                                                                                      | 120000         |
| Work Experience (years)                                                                                                                                                                                     | 8              |
| Credit Utilisation Rate (%)                                                                                                                                                                                 | 70             |
| Debt to Income Ratio (%)                                                                                                                                                                                    | 21             |
| Delinquencies (last 2 years)                                                                                                                                                                                | 0              |
| <b>DECISION:</b>                                                                                                                                                                                            | <b>APPROVE</b> |

TABLE VI  
CREDIT SCENARIO 2

| Applicant Profile                                                                                                                                                                                                              |                |
|--------------------------------------------------------------------------------------------------------------------------------------------------------------------------------------------------------------------------------|----------------|
| Feature                                                                                                                                                                                                                        | Value          |
| Loan Amount (\$)                                                                                                                                                                                                               | 11000          |
| Loan Term (months)                                                                                                                                                                                                             | 36             |
| Interest Rate (%)                                                                                                                                                                                                              | 16.5           |
| Credit Rating                                                                                                                                                                                                                  | C              |
| Salary                                                                                                                                                                                                                         | 28000          |
| Work Experience (years)                                                                                                                                                                                                        | 4              |
| Credit Utilisation Rate (%)                                                                                                                                                                                                    | 43.4           |
| Debt to Income Ratio (%)                                                                                                                                                                                                       | 7.35           |
| Delinquencies (last 2 years)                                                                                                                                                                                                   | 0              |
| <b>DECISION:</b>                                                                                                                                                                                                               | <b>APPROVE</b> |
| Your details were supplied to a credit-scoring algorithm that decided to approve your loan application based on your credit rating of C.                                                                                       |                |
| <b>Counterfactual explanation:</b> We would have DENIED you the loan if your credit rating was worse than your current credit rating. If your credit rating score had been between D and F, we would have denied you the loan. |                |
| <b>Directive explanation:</b> We would have DENIED you the loan if your credit rating score was between D and F. If you missed your monthly credit card payments for six months, your credit rating will be D or worse.        |                |
| <b>Prototypical explanation:</b> The following is an example of a DENIED applicant:                                                                                                                                            |                |
| Applicant Profile                                                                                                                                                                                                              |                |
| Feature                                                                                                                                                                                                                        | Value          |
| Loan Amount (\$)                                                                                                                                                                                                               | 7700           |
| Loan Term (months)                                                                                                                                                                                                             | 60             |
| Interest Rate (%)                                                                                                                                                                                                              | 19.29          |
| Credit Rating                                                                                                                                                                                                                  | E              |
| Salary                                                                                                                                                                                                                         | 36000          |
| Work Experience (years)                                                                                                                                                                                                        | 1              |
| Credit Utilisation Rate (%)                                                                                                                                                                                                    | 30             |
| Debt to Income Ratio (%)                                                                                                                                                                                                       | 83             |
| Delinquencies (last 2 years)                                                                                                                                                                                                   | 1              |
| <b>DECISION:</b>                                                                                                                                                                                                               | <b>DENY</b>    |

TABLE VII  
CREDIT SCENARIO 3

| Applicant Profile                                                                                                                                                                                                                               |                |
|-------------------------------------------------------------------------------------------------------------------------------------------------------------------------------------------------------------------------------------------------|----------------|
| Feature                                                                                                                                                                                                                                         | Value          |
| Loan Amount (\$)                                                                                                                                                                                                                                | 3000           |
| Loan Term (months)                                                                                                                                                                                                                              | 36             |
| Interest Rate (%)                                                                                                                                                                                                                               | 15.6           |
| Credit Rating                                                                                                                                                                                                                                   | C              |
| Salary                                                                                                                                                                                                                                          | 30000          |
| Work Experience (years)                                                                                                                                                                                                                         | 8              |
| Credit Utilisation Rate (%)                                                                                                                                                                                                                     | 29             |
| Debt to Income Ratio (%)                                                                                                                                                                                                                        | 16.44          |
| Delinquencies (last 2 years)                                                                                                                                                                                                                    | 0              |
| <b>DECISION:</b>                                                                                                                                                                                                                                | <b>APPROVE</b> |
| Your details were supplied to a credit-scoring algorithm that approved your loan application based on your credit utilisation rate of 29%.                                                                                                      |                |
| <b>Counterfactual explanation:</b> We would have DENIED you the loan if your credit utilisation rate was worse than your current utilisation rate. If your credit utilisation rate had been higher than 30%, we would have denied you the loan. |                |
| <b>Directive explanation:</b> We would have DENIED you the loan if your credit utilisation rate was higher than 30%. If you kept on using your credit card without paying them off, you could increase your credit utilisation rate to 30       |                |
| <b>Prototypical explanation:</b> The following is an example of a DENIED applicant:                                                                                                                                                             |                |
| Applicant Profile                                                                                                                                                                                                                               |                |
| Feature                                                                                                                                                                                                                                         | Value          |
| Loan Amount (\$)                                                                                                                                                                                                                                | 7700           |
| Loan Term (months)                                                                                                                                                                                                                              | 60             |
| Interest Rate (%)                                                                                                                                                                                                                               | 19.29          |
| Credit Rating                                                                                                                                                                                                                                   | E              |
| Salary                                                                                                                                                                                                                                          | 36000          |
| Work Experience (years)                                                                                                                                                                                                                         | 1              |
| Credit Utilisation Rate (%)                                                                                                                                                                                                                     | 30             |
| Debt to Income Ratio (%)                                                                                                                                                                                                                        | 83             |
| Delinquencies (last 2 years)                                                                                                                                                                                                                    | 1              |
| <b>DECISION:</b>                                                                                                                                                                                                                                | <b>DENY</b>    |

TABLE VIII  
CREDIT SCENARIO 4
